# Supplementary material for: Dimension Agnostic Neural Processes
Source: arXiv:2502.20661 source file (2025-02-28)
Supplement: Supplementary file 1 [file ablationstudy.tex]

\section{Ablation Study}
\label{app:sec:ablation_study}
\begin{table}[t]
    \caption{Context and target log likelihood values on data sampled from Gaussian Processes with various kernel. Here we trained the same model with different losses. Performances are measured over 4 seeds.\\}
    \label{tab:table_gp_inf_ablation}
    \centering
    \scriptsize
    
    \resizebox{0.95\textwidth}{!}{
    \begin{tabular}{lrrrrrrrrrrrr}
        \toprule
        \multirow{3}{*}{Model} & \multicolumn{2}{r}{RBF}                                   & \multicolumn{2}{r}{Matern}                                & \multicolumn{2}{r}{Periodic}                                & \multicolumn{2}{r}{$t$-noise}                               \\
                                 \cmidrule(lr){2-3}                                          \cmidrule(lr){4-5}                                          \cmidrule(lr){6-7}                                            \cmidrule(lr){8-9}
                               & context                     & target                      & context                     & target                      & context                      & target                       & context                      & target                       \\
        \midrule
MPNP (ours)                                              &         1.086  $\pm{0.005}$ &         0.457  $\pm{0.002}$ &         1.005  $\pm{0.014}$ &         0.278  $\pm{0.006}$ &         -0.017  $\pm{0.013}$ &         -0.681  $\pm{0.009}$ &          0.119  $\pm{0.025}$ &         -0.381  $\pm{0.013}$ \\
- $\calL_{\text{amort}}$                                 &         1.146  $\pm{0.010}$ &         0.487  $\pm{0.009}$ &         1.064  $\pm{0.002}$ &         0.300  $\pm{0.005}$ &         -0.002  $\pm{0.039}$ &         -0.673  $\pm{0.011}$ &          0.166  $\pm{0.027}$ &         -0.372  $\pm{0.043}$ \\
- $\calL_{\text{pseudo}}$                                &         1.090  $\pm{0.008}$ &         0.445  $\pm{0.006}$ &         1.012  $\pm{0.004}$ &         0.277  $\pm{0.007}$ &          0.058  $\pm{0.018}$ &         -0.669  $\pm{0.007}$ &          0.239  $\pm{0.006}$ &         -0.348  $\pm{0.023}$ \\
- $\calL_{\text{amort}}$ - $\calL_{\text{pseudo}}$       &         1.160  $\pm{0.008}$ &         0.493  $\pm{0.006}$ &         1.092  $\pm{0.012}$ &         0.320  $\pm{0.004}$ &          0.074  $\pm{0.019}$ &         -0.666  $\pm{0.010}$ &          0.365  $\pm{0.010}$ &         -0.416  $\pm{0.086}$ \\
\cmidrule(lr){1-1}       \cmidrule(lr){2-3}                                          \cmidrule(lr){4-5}                                          \cmidrule(lr){6-7}                                            \cmidrule(lr){8-9}
MPANP (ours)                                             &         1.374  $\pm{0.000}$ &         0.698  $\pm{0.007}$ &         1.373  $\pm{0.001}$ &         0.501  $\pm{0.005}$ &          1.153  $\pm{0.049}$ &         -0.638  $\pm{0.030}$ &          0.773  $\pm{0.039}$ &         -0.446  $\pm{0.057}$ \\
- $\calL_{\text{amort}}$                                 &         1.359  $\pm{0.001}$ &         0.703  $\pm{0.001}$ &         1.351  $\pm{0.006}$ &         0.501  $\pm{0.004}$ &          1.007  $\pm{0.064}$ &         -0.651  $\pm{0.032}$ &          0.496  $\pm{0.023}$ &         -0.520  $\pm{0.059}$ \\
- $\calL_{\text{pseudo}}$                                &         1.375  $\pm{0.000}$ &         0.678  $\pm{0.010}$ &         1.373  $\pm{0.002}$ &         0.480  $\pm{0.007}$ &          1.129  $\pm{0.065}$ &         -0.606  $\pm{0.005}$ &          0.786  $\pm{0.056}$ &         -0.433  $\pm{0.011}$ \\
- $\calL_{\text{amort}}$ - $\calL_{\text{pseudo}}$       &         1.374  $\pm{0.001}$ &         0.680  $\pm{0.002}$ &         1.370  $\pm{0.007}$ &         0.486  $\pm{0.014}$ &          0.811  $\pm{0.142}$ &         -0.789  $\pm{0.132}$ &          0.826  $\pm{0.030}$ &         -0.428  $\pm{0.037}$ \\
        \bottomrule
    \end{tabular}}
\end{table}

\begin{figure}[t]
    \centering
    \includegraphics[width = 0.32\textwidth]{figure/sample plot 9 amort.pdf}
    \includegraphics[width = 0.32\textwidth]{figure/sample plot 9 pseudo.pdf}
    \includegraphics[width = 0.32\textwidth]{figure/sample plot 9 both.pdf}
    \caption{Generated pseudo context data samples of MPANP in 1d regression task. (Left) Generated pseudo context when we remove the term $\calL_{\text{amort}}$ from the loss $\calL$. (Middle) Generated pseudo context when we remove the term $\calL_{\text{pseudo}}$ from the loss $\calL$. (Right) Generated pseudo context when we remove the terms $\calL_{\text{amort}}$ and $\calL_{\text{pseudo}}$ from the loss $\calL$.} 
    \label{fig:feature_ablation}
\end{figure}

In this section, we conduct some ablation studies on loss function and report the generated pseudo context data and the performances of the \glspl{mpnp} in 1D regression.
As our loss function essentially contain the $\calL_{\text{marg}}$ term, we conduct the ablation studies on the other terms ($\calL_{\text{pseudo}}$ and $\calL_{\text{amort}}$). 
We have three cases i) loss function $\calL$ without $\calL_{\text{amort}}$, ii) loss function $\calL$ without $\calL_{\text{pseudo}}$ and iii) loss function $\calL$ without $\calL_{\text{amort}}$ and $\calL_{\text{pseudo}}$.
We report the performances of the three cases in \cref{tab:table_gp_inf_ablation}.
Also we present the generated pseudo context data from the three cases in \cref{fig:feature_ablation}.
Here you can see that without any term in $\calL$, the model cannot actually generate meaningful pseudo context dataset from real context dataset.
