# Supplementary material for: Dimension Agnostic Neural Processes
Source: arXiv:2502.20661 source file (2025-02-28)
Supplement: Supplementary file 2 [file directlygeneratinginput.tex]

\section{Directly Generating Input Model}
\label{app:sec:directly_generating_input}
In this section, we present our model generating pseudo contexts directly in the input space.
We will present two kinds of model structure, i) directly generating pseudo context pair $(x,y)$ simultaneously by ISAB, ii) generating pseudo context data $x$ and $y$, sequentially. 
\subsection{Construction}
\paragraph{Generating pseudo context pair simultaneously.}
The generator of our first model which simultaneously generating pseudo context pair $(x',y')$, takes real context dataset $Z_c$ as input and outputs pseudo context dataset $Z'$. 
Here the generator is the one layer ISAB module.
Then we concatenate $Z_c$ and $Z'$ in order to treat this concatenated set as context dataset.
Then the encoder takes this concatenated context set as input.
And the others are the same with \gls{cnp} or \gls{canp}.
\paragraph{Sequentially generating pseudo context data \texorpdfstring{$x$}{x} and \texorpdfstring{$y$}{y}}
In this model, the generator takes real context dataset $Z_c$ as input and outputs only $x'$s of $Z'$. 
Here the generator is the one layer ISAB module with additional one linear layer.
Then we consider these $x'$s as our target dataset and find the mean and variance of $y'$ for each $x'$ by forwarding the model with context dataset $Z_c$ and target $x'$.
We sample $y'$ from the Gaussian distribution with mean and variance from the prior step.
We again concatenate $Z_c$ with $Z'$ and use them as context dataset.
\subsection{Sample}
\begin{figure}[t]
    \centering
    \includegraphics[width = 0.32\textwidth]{figure/sample plot 9 xy without pseudo.pdf}
    \includegraphics[width = 0.32\textwidth]{figure/sample plot 9 xy.pdf}
    \includegraphics[width = 0.32\textwidth]{figure/sample plot 9 residual.pdf}
    \caption{Generated pseudo context data samples of MPANP in 1d regression task. (Left) Generated pseudo context samples from simultaneously generating model without the term $\calL_{\text{amort}}$ in the loss $\calL$. (Middle) Generated pseudo context samples from simultaneously generating model after adding the term $\calL_{\text{amort}}$ in the loss $\calL$. (Right) Generated pseudo context samples from sequentially generating model.} 
    \label{fig:direct}
\end{figure}
In this section, we presents how the directly generating input model actually samples the pseudo context datasets. 
In \cref{fig:direct}, we report generated pseudo context dataset from three different cases of directly generating input model.
The first figure on the left of the \cref{fig:direct} shows the generated pseudo context samples from simultaneously generating model without the term $\calL_{\text{amort}}$ in the loss $\calL$.
Here, we can see that the generator learns to generate meaningless inputs that are ignored by the decoder.
The second figure on the middle of the \cref{fig:direct} shows the generated pseudo context samples from simultaneously generating model after adding the term $\calL_{\text{amort}}$ in the loss $\calL$.
In this figure, we can see that although the model generates much more meaningful pseudo context dataset compare to the first one, still the generator fails to make sufficiently reasonable pseudo context dataset.
The third figure on the right of the \cref{fig:direct} shows the generated pseudo context samples from sequentially generating model.
In this figure, we can see that the model generates sufficiently meaningful pseudo context dataset compare to the others but it generates overconfidently for the unseen data points.
Thus it fails to capture the functional uncertainty of the model which occurs the lack of the performance.
% \subsection{Long Training}
